# Supplementary material for: Kernel-Level Energy-Efficient Neural Architecture Search for Tabular Dataset
Source: arXiv:2504.08359 source file (2025-04-11)
Supplement: Supplementary file 1 [file appendix.tex]

\subsection{Experiments on Intel NCS2}
Besides comparison experiments conducted on Jetson Nano, we also evaluate our proposed method with Intel NCS2 platforms. It is note-worthy that Intel NCS2 does not support operators dedicated for Transformer-based models. Table \ref{tab:5} shows the experimental results. Remarkably, both energy-aware NAS propose better models in terms of balance between energy efficiency and accuracy.

\begin{table*}[t]\scriptsize
    \centering
    \caption{A COMPARISION BETWEEN THE PROPOSED METHOD WITH OTHER BASELINES}
    \label{tab:5}
    \begin{tabular}{|c| c|c | c|c | c|c |}
    \hline
    \multirow{3}{*}{Benchmark}& \multicolumn{6}{c|}{\textbf{ResNet}}  \\
    \cline{2-7}
     & \multicolumn{2}{c|}{\textbf{Proposed NAS}} & \multicolumn{2}{c|}{ Conventional NAS} & \multicolumn{2}{c|}{Adapted-ETNAS} \\
    \cline{2-7}
    & \makecell[c]{Energy \\ (mJ)}  & Accuracy & \makecell[c]{Energy \\ (mJ)} & Accuracy & \makecell[c]{Energy \\ (mJ)} & Accuracy   \\
    \hline 
    \makecell[c]{BNA-UCI} & 0.866 & 0.997 & 9.354 & 1.0 & 0.891 & 0.997 \\ 
    \hline
    \makecell[c]{california} & 0.863 & 0.782 & 6.08 & 0.799 & 0.981 & 0.674\\
    \hline
    \makecell[c]{cpu\_small} & 0.867 & 0.927 & 10.035 & 0.969 & 0.988 & 0.917 \\
    \hline
    \makecell[c]{dataset\_sales} & 0.868 & 0.685 & 10.056 & 0.734 & 0.907 & 0.673  \\
    \hline
    \makecell[c]{EgyptianSkulls} & 0.87 & 0.205  &  10.709 & 0,288 & 1.911 & 0.134  \\
    \hline
    \makecell[c]{kin8nm} & 0.867 & 0.906 & 2.819 & 0.917 & 0.897 & 0.914 \\
    \hline
    \makecell[c]{liver-disorders} & 0.881 & 0.228 & 9.339 & 0.315 & 1.838 & 0.239 \\
    \hline
    \makecell[c]{mv} & 0.866 & 0.998 & 8.452 & 1.0 & 0.877 & 1.0 \\
    \hline
    \makecell[c]{Wine} & 0.867 & 0.374 & 7.179 & 0.396 & 0.917 & 0.373 \\
    \hline
    \makecell[c]{MISO} & 0.866 & 0.982 & 6.933 & 0.986 & 0.887 & 0.984 \\
    \hline
    \end{tabular}
    \begin{tabular}{|c| c|c | c|c | c|c |}
    \hline
    \multirow{3}{*}{Benchmark}& \multicolumn{6}{c|}{\textbf{MLP}}  \\
    \cline{2-7}
     & \multicolumn{2}{c|}{\textbf{Proposed NAS}} & \multicolumn{2}{c|}{ Conventional NAS} & \multicolumn{2}{c|}{Adapted-ETNAS}  \\
    \cline{2-7}
    & \makecell[c]{Energy \\ (mJ)}  & Accuracy & \makecell[c]{Energy \\ (mJ)} & Accuracy & \makecell[c]{Energy \\ (mJ)} & Accuracy  \\
    \hline 
    \makecell[c]{BNA-UCI} & 0.520 & 0.998 & 5,191 & 1.0 & 0.533 & 0.905  \\ 
    \hline
    \makecell[c]{california} & 0.521 & 0.668 & 5.092 & 0.675 & 0.533 & 0.624 \\
    \hline
    \makecell[c]{cpu\_small} & 0.519 & 0.75 & 5.139 & 0.922 & 0.528 & 0.769 \\
    \hline
    \makecell[c]{dataset\_sales} &  0.521 & 0.658 & 3.313 & 0.65 & 0.532 & 0.677  \\
    \hline
    \makecell[c]{EgyptianSkulls} & 0.524 & 0.299 & 3.288 & 0.288 &0.531  & 0.265  \\
    \hline
    \makecell[c]{kin8nm} & 0.523 & 0.918 & 2.36 & 0.937 & 0.531 & 0.926 \\
    \hline
    \makecell[c]{liver-disorders} & 0.524 & 0.219 & 3.3 & 0.221 & 0.531 & 0.209 \\
    \hline
    \makecell[c]{mv} & 0.518 & 0.997 & 1.366 & 1.0 & 0.533 & 1.0 \\
    \hline
    \makecell[c]{Wine} & 0.523 & 0.351 & 2.381 & 0.384 & 0.533 & 0.373\\
    \hline
    \makecell[c]{MISO} & 0.518 & 0.983 & 1.578 & 0.989 & 0.533 & 0.905 \\
    \hline
    \end{tabular}
\end{table*}

% \subsection{Determine Energy-efficient GPU clock frequency for inference phase}
